# Supplementary material for: Ion native variational ansatz for quantum approximate optimization
Source: arXiv:2206.11908 source file (2022-06-23)
Supplement: Supplementary file 1 [file appendix_ion_model_ham.tex]

In trapped ion coulomb crystals, different types of spin-spin interactions can be implemented upon application of different external fields \cite{Monroe2021}. Here we focus on the long range Ising couplings 
given by the Eqs.~\eqref{eq:ising_hamiltonian} and  \eqref{eq:ion_ising_couplings}. 
Such an effective Hamiltonian arises when the ions are illuminated 
by bichromatic laser beams with the
same wavelengths but different intensities. 
The beams off-resonantly couple the ion qubits with the collective motional modes. 
With knowledge of the motional modes
normal vectors 
%$b_{j\alpha}$ 
and frequencies,
%$\omega_{\alpha}$ (where $j$ and $\alpha$ are the ion number
%and the phonon mode number correspondingly)
the spin coupling matrix can be
calculated as follows \cite{Jurcevic2014}:
\begin{equation}
  J_{jk} = \Omega_{j}\Omega_k \frac{\hbar k^2}{2m} \sum_\alpha \frac{b_{j\alpha}b_{k\alpha}}{\Delta^2 - \omega_\alpha^2},
\end{equation}
where $\Omega_{j}$ are Rabi frequencies of the field acting 
on ion number $j$, $\alpha$ enumerates the  phonon modes,
$\omega_\alpha$ and $b_{i\alpha}$ are the phonon modes frequencies and 
normal vectors, 
$\Delta$ is the detuning of the lasers frequency from the qubit transition,
$m$ is the ions mass and $k$ is the wavevector of 
the field acting on the ions.

At arbitrary detunings, $J_{jk}$ can have
complex dependence on $j$ and $k$. 
However, at
certain values of $\Delta$ 
(when the detuning slightly exceeds
the frequency of the radial COM mode), the dependence
of $J_{jk}$ on $j$ and $k$ can be approximated with the power law
$1/|j-k|^r$ as in as in \eqref{eq:ion_ising_couplings}. The power
