# Supplementary material for: Ion native variational ansatz for quantum approximate optimization
Source: arXiv:2206.11908 source file (2022-06-23)
Supplement: Supplementary file 2 [file appendix_infidelity.tex]

\newpage
\appendix

\section{}

Consider the classical fidelity $F$ between the true $c=(\begin{array}{lr}\sqrt{p} & \sqrt{1-p}\end{array})^T$ and the reconstructed   vectors. Classical fidelity is related to the so-called Hellinger distance in classical statistics \cite{Borovkov1999}. 

Using the Fisher information matrix and Cram\'er--Rao bound one can show that the infidelity is asymptotically proportional to the chi--squared random variable with 1 degree of freedom \cite{bogdanov2004fundamental,bogdanov2009unified}:
\begin{equation*}
    1-F \sim d \cdot \xi^2,
\end{equation*}
where $\xi \sim N(0,1)$ is the standard normal random variable, $d=g/(4n)$, and $g$ is from \eqref{eq:var_factor}. From here one can see the increasing of infidelity by the factor of $g$ when the readout errors are present. However, one can eliminate that by increasing the sample size by the same factor.
